# Supplementary material for: Cycling tames power fluctuations near optimum efficiency
Source: arXiv:1805.00848 source file (2018-07-16)
Supplement: Supplementary file 1 [file SM.pdf]

# Supplemental Material
# Power fluctuations close to Carnot efficiency: Cyclic vs. steady state heat engines

Viktor Holubec[1,2,*] and Artem Ryabov[1]

[1] Charles University, Faculty of Mathematics and Physics,
Department of Macromolecular Physics, V Holešovičkách 2, 180 00 Praha 8, Czech Republic

[2] Universität Leipzig, Institut für Theoretische Physik, Postfach 100 920, D-04009 Leipzig, Germany

(Dated: July 16, 2018)

## WORK PDF FOR A QUASI-STATIC PROCESS

In this Section, we show that for any quasi-static process the PDF of work (defined through the time derivative of the Hamiltonian) converges to the delta function. The derivation generalizes the one given in Ref. [1] to any process $x(t)$, for which the PDF of $x(t)$ evolves according to the equation

$$\partial_t \rho(x,t) = \nu \mathcal{L}(t)[\rho(x,t)]. \tag{S1}$$

For a continuous Markovian dynamics the operator $\mathcal{L}(t)$ is a linear Fokker-Planck operator and for a discrete one it is a transition rate matrix. However, Eq. (S1) can also be a generalized Master equation for a non-Markovian process [2].

During the operational cycle of the engine, the evolution operator $\mathcal{L}(t)$ varies from $\mathcal{L}(0)$ to $\mathcal{L}(t_p)$ as both the temperature $T(t)$ and the Hamiltonian $H(x,t)$ change. Naturally, we assume that the system with the fixed Hamiltonian $H$ in contact with a heat bath at constant temperature $T$, will eventually relax to the Boltzmann distribution $\rho(x,\infty) = \rho_B(x) = \exp\left(-H/k_B T\right)/Z$, where $k_B$ denotes the Boltzmann constant and $Z$ is the partition function. The Boltzmann distribution thus satisfies $\mathcal{L}(t)[\rho_B(x,t)] = 0$. In Eq. (S1), the relaxation time to equilibrium is measured by the prefactor $\nu$. The relaxation is fast (slow) for $\nu$ large (small).

The process is quasi-static if the evolution operator $\mathcal{L}(t)$ changes on a time-scale much longer than the relaxation time. Since we are interested in finite-time processes only (in order to obtain a non-zero output power of the engine), we consider the limit of infinitely fast relaxation $\nu \to \infty$. At any instant $t$ during such a process, the PDF for $x$ is given by the Boltzmann distribution

$$\rho(x,t) \approx \rho_B(x,t) = \frac{1}{Z(t)} \exp\left[-\frac{H(x,t)}{k_B T(t)}\right], \tag{S2}$$

where $H(x,t)$ and $T(t)$ are values of the Hamiltonian and temperature at time $t$. Of course, the formula (S2) is in general valid only if the system is in contact with the heat bath. Once the bath is disconnected, the evolution becomes deterministic, determined by the specific form of the Hamiltonian. The formula (S2) is thus valid along the whole cycle with adiabatic branches of the type (ii), where the system never disconnects from the baths (see the main text). On the other hand, for systems with adiabatic branches of the type (i), where the system is disconnected from the bath, the formula (S2) holds during the isothermal branches only.

The work done by the system during the time interval $[0,t]$ is defined as

$$w(t) = -\int_0^t d\tau \dot{H}[x(\tau),\tau]. \tag{S3}$$

The dot denotes the partial derivative with respect to the time argument in $H(x,t)$, $\dot{H}(x,t) = \partial_t H(x,t)$. We will now derive the probability distribution for this stochastic functional assuming that the underlying stochastic process $x(t)$ is quasi-static with the PDF given by Eq. (S2).

The evolution equation for the joint probability density for $x(t)$ and $w(t)$ reads [2]

$$\partial_t \xi(x,w,t) = \dot{H}(x,t)\partial_w \xi(x,w,t) + \nu \mathcal{L}(x,t)[\xi(x,w,t)]. \tag{S4}$$

The desired PDF for work, $p(w,t)$, obtained from $\xi(x,w,t)$ by integration over $x$, $p(w,t) = \int dx \xi(x,w,t)$, obeys the evolution equation

$$\partial_t p(w,t) = \int dx \dot{H}(x,t)\partial_w \xi(x,w,t) + \int dx \nu \mathcal{L}(t)[\xi(x,w,t)]. \tag{S5}$$

The equation cannot be solved in general and its solution is known only in a few special cases [1]. Nevertheless, we are interested only in the quasi-static limiting case $\nu \to \infty$, where the equation can be solved by the Ansatz $\xi(x,w,t) \approx \rho_B(x,t) p(w,t)$. After inserting the Ansatz into Eq. (S5), the last term on the right-hand side vanishes due to the quasi-static condition $\mathcal{L}(t)[\rho_B(x,t)] = 0$, and Eq. (S5) reduces to the pure convection equation

$$\partial_t p(w,t) = \left[\int dx \dot{H}(x,t)\rho_B(x,t)\right] \partial_w p(w,t). \tag{S6}$$

Solution to this convection equation is

$$p(w,t) = \delta(w - W(t)), \tag{S7}$$

where $\delta$ denotes the Dirac $\delta$-function and

$$W(t) = -\int_0^t d\tau \int dx \dot{H}(x,\tau)\rho_B(x,\tau) \tag{S8}$$

is the average work done by the system during the quasi-static process.

## DERIVATION OF FORMULAS (3)–(5) FOR CYCLIC HEAT ENGINES

In this Section, we derive the formulas (3)–(5) in the main text for the stochastic work $w = -\int_0^{t_p} dt\dot{H}(x(t),t)$ done by periodically driven heat engines (HEs) disconnected from the reservoirs during the adiabatic branches. The considered Carnot cycle is quasi-static and the PDF for $w$ can be calculated solely using the Boltzmann distribution (S2).

Due to the self-averaging property of work done during quasi-static processes where the system is in contact with the reservoirs, which we described in the preceding section, the work PDFs for the isothermal branches are given by $\delta$-functions located at the positions of the reversible works. For the hot isotherm, the reversible work can be calculated using the combination of the first and the second law of thermodynamics in the form $W_1 = T_h\Delta S - \langle \Delta H_1\rangle$, where $\Delta S = \Delta S_1$ and $\langle \Delta H_1\rangle$ denote the change of the system entropy and the change of the average internal energy of the system during the hot isotherm, respectively. The reversible work done during the cold isotherm can be calculated along similar lines. It reads $W_3 = -T_c\Delta S - \langle \Delta H_3\rangle$. The minus sign before the entropy term follows from the fact that the change of the system entropy during the cold isotherm is given by $\Delta S_3 = -\Delta S$ as follows from the condition that the change of the system entropy per cycle, $\Delta S_1 + \Delta S_3$, vanishes. To sum up, the PDF for work done along the hot isotherm reads $p_1(w) = \delta(w - W_1)$ and the one for the cold isotherm is given by $p_3(w) = \delta(w - W_3)$.

During the adiabatic branches when the reservoir is disconnected from the system, the work lacks the self averaging property of quasi-static processes which slightly complicates the calculation of the corresponding PDFs. Since no heat can be interchanged during such adiabats, the stochastic work done during the adiabats is simply given by the decrease of the internal energy along these branches. Concretely, we get $w_2 = -\Delta H_2$ for the first adiabat and $w_4 = -\Delta H_4$ for the second one. The PDFs for these works are thus determined by the PDFs for the changes of energy. Formally, we can write the work PDF for the first adiabat as $p_2(w) = \langle \delta(w + \Delta H_2)\rangle$ and as $p_4(w) = \langle \delta(w + \Delta H_4)\rangle$ for the second one. These averages must by taken over the PDFs for $\Delta H_2$ and $\Delta H_4$, respectively. Due to the quasi-staticity of the considered cycle, these PDFs are independent and can be constructed from the Boltzmann distribution (S2).

For infinitely fast adiabatic branches the microstate of the system does not change during the adiabats. Assuming that the system dwells in a microstate $x$ at the beginning of the first adiabat and at a microstate $y$ at the beginning of the second one, the changes of the internal energy are given by $\Delta H_2 = H(x, t_1 + t_2) - H(x, t_1)$ and $\Delta H_4 = H(x, t_p) - H(x, t_p - t_4)$, where $t_i$, $i = 1, \dots, 4$ denote durations of the individual branches (see Fig. 1 in the main text). In this case, the average in the PDF $p_2(w)$ must be calculated over the PDF $\rho_B(x, t_1) = \rho_B(x, t_1 + t_2)$ and the one in $p_4(w)$ over the PDF $\rho_B(x, t_p - t_4) = \rho_B(x, t_p)$.

If the reservoirs are disconnected from the system for a finite time interval, the system microstate and thus also the corresponding PDF during the adiabatic branches deterministically changes. In order to avoid bringing the system out of equilibrium after the ends of such adiabats, the driving must be chosen in such a way that the PDF for $x$ just before the end of an adiabat is equivalent to the equilibrium PDF corresponding to the Hamiltonian and bath temperature after reconnecting the system and the bath when the adiabat ends. Let us denote as $x_2$ the microstates occupied at the beginning of the first adiabat. Because the system evolution during the adiabat is deterministic, the microstate at its end, $y_2 = y_2(x_2)$, is a function of $x_2$. The corresponding change of the internal energy reads $\Delta H_2 = H(y_2(x_2), t_1 + t_2) - H(x_2, t_1)$ and the average in the PDF $p_2(w)$ must be calculated over the PDF $\rho_B(x_2, t_1)$. To get explicit results, it is necessary to know the specific form of the mapping $y_2(x_2)$, i.e. to solve concrete dynamical equations for the microstate during the adiabat.

To avoid this, we here consider two situations which can be treated without specifying the dynamics. First, one can drive the system in such a way that $y_2(x_2) = x_2$, and return to the situation of infinitely fast adiabatic branches. Second, one can use the approximation that $x_2$ and $y_2$ are independent of each other. In this case, the average in the PDF $p_2(w)$ must be calculated over the PDF $\rho_B(x_2, t_1)\rho_B(y_2, t_1 + t_2)$. Using similar notation, the change of the internal energy during the second adiabat can be written as $\Delta H_4 = H(y_4, t_p) - H(x_4, t_p - t_4)$. If we again use the approximation that $x_4$ and $y_4$ are independent, the average in the PDF $p_4(w)$ must be calculated over the PDF $\rho_B(x_4, t_p - t_4)\rho_B(y_4, t_p)$.

The work PDF for the whole cycle is given by the convolution of the work PDFs for the individual branches, $p(w) = p_1 \star p_2 \star p_3 \star p_4(w) = \langle \delta\left\{w - [W_1 + W_2 - \Delta H_2 - \Delta H_4]\right\}\rangle$. Using the condition on zero change of the system average internal energy per cycle, $\sum_{i=1}^4 \langle \Delta H_i\rangle = 0$, the expression $W_1 + W_2 - \Delta H_2 - \Delta H_4$ can be rewritten as $(T_h - T_c)\Delta S - (\Delta H_2 - \langle \Delta H_2\rangle) - (\Delta H_4 - \langle \Delta H_4\rangle)$. The PDF for the work done per cycle thus reads

$$p(w) = \left\langle \delta\left\{ w - \left[ W - \widetilde{\Delta H}_2 - \widetilde{\Delta H}_4 \right] \right\} \right\rangle, \qquad \text{(S9)}$$

where $\widetilde{\Delta H}_i = \Delta H_i - \langle \Delta H_i\rangle$, $i = 2, 4$ and $W = (T_h - T_c)\Delta S$. Integrals over this function yield all moments of work: $\langle w^m\rangle = \int_{-\infty}^{\infty} dw w^m p(w)$. The first one ($m = 1$) is

given by

$$\langle w \rangle = W = (T_h - T_c)\Delta S \tag{S10}$$

and the second one ($m = 2$) reads

$$\left\langle w^2 \right\rangle = W^2 + \left\langle \Delta H_2^2 \right\rangle - \left\langle \Delta H_2 \right\rangle^2 + \left\langle \Delta H_4^2 \right\rangle - \left\langle \Delta H_4 \right\rangle^2 . \tag{S11}$$

Equations (S9)–(S11) are valid for an arbitrary Carnot cycle with adiabatic branches where the system and reservoir are disconnected. To get specific expressions for specific models, the averages must be taken over the proper PDFs for $\Delta H_2$ and $\Delta H_4$, as described above.

For the instantaneous adiabatic branches, the changes in the internal energy assumes the form $\Delta H_2 = H(x, t_1 + t_2) - H(x, t_1)$ and $\Delta H_4 = H(y, t_p) - H(y, t_p - t_4)$ and the averages must be taken over the PDF $\rho_B(x, t_1)\rho_B(y, t_p)$. Using the Hamiltonian $H(x, t) = k(t)x^{2n}/2n$, Eqs. (S10) and (S11) gives the work variance

$$\sigma_w^2 = \left\langle w^2 \right\rangle - W^2 = \frac{k_B^2}{n}(T_h - T_c)^2 \tag{S12}$$

which, together with $W = (T_h - T_c)\Delta S$, implies Eq. (4) in the main text for the work fluctuation.

For the finite time adiabats, under the assumption that the microstates occupied at the beginnings and at the ends of the adiabats are independent, the changes in the internal energy assumes the form $\Delta H_2 = H(y_2, t_1 + t_2) - H(x_2, t_1)$ and $\Delta H_4 = H(y_4, t_p) - H(x_4, t_p - t_4)$ and the averages must be taken over the PDF $\rho_B(x_2, t_1)\rho_B(y_2, t_1 + t_2)\rho_B(x_4, t_p - t_4)\rho_B(y_4, t_p)$. Using the Hamiltonian $H(x, t) = k(t)x^{2n}/2n$, we obtain from Eqs. (S10) and (S11) the formula

$$\sigma_w^2 = \frac{k_B^2}{n}(T_h + T_c)^2 \tag{S13}$$

for the work variance and the formula (5) in the main text for the work fluctuation.

## CYCLIC BROWNIAN HEAT ENGINE

The HE is based on an overdamped Brownian particle diffusing in a harmonic potential

$$U(x, t) = H(x, t) = k(t)x^2/2. \tag{S14}$$

Its position $x = x(t)$ obeys the Langevin equation

$$\dot{x} = -kx/\gamma + \sqrt{2k_B T/\gamma}\zeta. \tag{S15}$$

Here, $\gamma$ is the friction coefficient and $\zeta$ is the Gaussian white noise with $\langle \zeta \rangle = 0$ and $\langle \zeta(t)\zeta(t') \rangle = \delta(t - t')$. The bath temperature $T$ and the stiffness $k$ are varied along the Carnot cycle depicted in Fig. 1 in the main text. Specifically, we use the stiffness protocol

$$k(t) = \begin{cases} \frac{1}{\sigma_0^2}\frac{k_B T_h}{(1+b_1 t)^2} - \frac{\gamma b_1}{1+b_1 t}, & t \in [0, t_1), \\ \frac{1}{\sigma_f^2}\frac{k_B T_c}{[1+b_2(t-t_1)]^2} - \frac{\gamma b_2}{1+b_2(t-t_1)}, & t \in [t_1, t_p), \end{cases} \tag{S16}$$

maximizing the work done by the engine per cycle once the system entropy change during the hot isotherm $\Delta S = k_B \log \sigma_f/\sigma_0$ and durations $t_1$ and $t_3$ of the two isotherms are fixed [3, 4]. In Eq. (S16), the parameter $\sigma_0^2$ ($\sigma_f^2$) stands for the variance of the particle position at the beginning (end) of the hot isotherm. The adiabatic branches are assumed to be instantaneous ($t_2 = t_4 = 0$) and thus $t_p = t_1 + t_3$ denotes the duration of the whole cycle. The constants $b_1$ and $b_2$ are given by $b_1 = (\sigma_f/\sigma_0 - 1)/t_1$ and $b_2 = (\sigma_0/\sigma_f - 1)/t_3$. For $t_1$ and $t_3$ much larger than the system relaxation time $\tau_x = k/\gamma$, the driving produces a quasi-static process even though it changes infinitely fast during the adiabats. This is because the jumps of the stiffness during these branches balance the jumps in the temperature keeping constant the ratio $k/T$ and thus also the equilibrium position distribution $\rho(x) = \exp(-kx^2/2k_B T)/Z_x$.

Besides the protocol (S16) is optimal, it also leads to concise expressions for power and efficiency [3, 5]

$$P = \frac{(T_\mathrm{h} - T_\mathrm{c})\Delta S}{t_p} - \frac{A}{t_1 t_p} - \frac{A}{t_3 t_p}, \tag{S17}$$

$$\eta = \frac{W_\mathrm{out}}{Q_\mathrm{h}} = \frac{\eta_\mathrm{C}}{1 + T_\mathrm{c}\Delta S_\mathrm{tot}/W}, \tag{S18}$$

where the parameter $A = \gamma\left(\sigma_f - \sigma_0\right)^2$ measures the work dissipated due to the irreversible realization of the cycle for $t_1 \approx t_3 \approx \tau_x$ and the entropy produced per cycle $\Delta S_\mathrm{tot} = A(1/T_h t_1 + 1/T_c t_3)$ assumes the so called low-dissipation form [3, 6]. General calculation of the work/power fluctuation $\tilde{\sigma}_w$ is more involved. One can either calculate it with the help of Brownian dynamics simulation of the Langevin equation, or numerically, for example using the method suggested in Ref. [7]. We use the analytical method presented in Ref. [4].

In the considered setting, the Carnot efficiency is reached in the limit of infinitely fast cycles with infinitely strong driving [8]. More precisely, introducing the scaling

$$\sigma_f \propto \sigma_\infty^{-\xi}, \quad t_p \propto \sigma_\infty^{(\chi-1)\xi} \tag{S19}$$

while keeping constant the ratio $\sigma_f/\sigma_0 > 0$ yields in the limit $\sigma_\infty$ the Carnot efficiency at a nonzero power for $\xi > 0$ and $\chi \in (0, 1]$. Under the scaling (S19) the position relaxation time $\tau_x = \gamma/k \propto \sigma_\infty^{-\xi}$ vanishes faster than the cycle duration $t_p \propto \sigma_\infty^{(\chi-1)\xi}$, and thus, although fast, the cycle can be regarded as quasi-static. Different from the shortcuts to adiabaticity and equilibrium presented in the literature [9–13], the fast relaxation is caused by decreasing the system relaxation time $\tau_x$ by increasing the stiffness $k$ rather than by devising a clever protocol.

| $t_p$ | $\langle w\rangle$ | $\langle w^2\rangle$ | $P$ | $\langle P^2\rangle$ | $\Delta S_{tot}$ | $\Delta S_{tot}/t_p$ | $\eta_C - \eta$ |
|---|---|---|---|---|---|---|---|
| $\sigma_\infty^{(\chi-1)\xi}$ | $\sigma_\infty^0$ | $\sigma_\infty^0$ | $\sigma_\infty^{(1-\chi)\xi}$ | $\sigma_\infty^{2(1-\chi)\xi}$ | $\sigma_\infty^{-\chi\xi}$ | $\sigma_\infty^{(1-2\chi)\xi}$ | $\sigma_\infty^{-\chi\xi}$ |

TABLE I. Scalings of the main variables in the Brownian HE with the harmonic Hamiltonian (S14). The engine can work with the Carnot efficiency at nonzero power with finite fluctuation whenever $\xi > 0$ and $\chi \in (0, 1]$.

In Tab. I, we sum scalings of the most important parameters of the Brownian HEs with $\sigma_\infty$. Let us note that the cycle duration $t_p^\star$, corresponding to the maximum power $P^\star$ attainable in the HE once all its parameters except for $t_p$ are fixed, scales as $1/k$ and thus it is proportional to the position relaxation time $\tau_x$. Interestingly, the maximum power $P^\star$ is always much larger than $P$ at $\eta_C$ [8].

According to Ref. [8], the overdamped Brownian HEs work with $\eta = \eta_C$ and $P > 0$ whenever they operate in the low-dissipation regime, where the work dissipated during the hot (cold) isotherm scales as $1/t_1$ $(1/t_3)$. This is achieved if the state of the system depends during the hot (cold) isotherm on time solely through the combination $t/t_1$ $(t/t_3)$. In fact, the Carnot bound at $P > 0$ can be reached under much milder conditions of: 1) Short cycle times $t_p$ which are nevertheless long compared to the relaxation times for position $\tau_x$ and for the momentum $\tau_p = m/\gamma$. In practice, the time-scale separation $t_p \gg \tau_x, \tau_p$ must be realized in such a way that the time-scales $\tau_x$ and $\tau_p$ are much larger than the reservoir relaxation time [14]. 2) Driving leading to nonzero reversible work $W = (T_\mathrm{h} - T_\mathrm{c})\Delta S$. 3) A Carnot cycle composed of two adiabats and two isotherms.

The curves plotted in Fig. 2 in the main text are calculated for a round glass particle with the density $\rho_g = 2800$ kg/m$^3$ and radius $R = 10^{-6}$ m diffusing in water with dynamical viscosity $\kappa = 0.001$ Pa s, which is assumed to be temperature independent. The friction coefficient $\gamma = 6\pi R\kappa$, is calculated according to the Stokes law. We take $\sigma_f = \sigma_\infty^{-\xi}$ and $\sigma_f^2/\sigma_0^2 = 3$ for the boundary variances, $t_1 = t_3 = t_p/2$ for durations of the isothermal branches, $T_c = 293.15$ K and $T_h = 5273.15$ K for the reservoir temperatures and $\xi = 1.5$ and $\chi = 0.05$ for the exponents defined in Eq. (S19).

* viktor.holubec@gmail.com


[1] V. Holubec, *Non-equilibrium Energy Transformation Processes*, Springer Theses (Springer International Publishing, 2014).

[2] T. Speck and U. Seifert, Journal of Statistical Mechanics: Theory and Experiment **2007**, L09002 (2007).

[3] T. Schmiedl and U. Seifert, EPL **81**, 20003 (2008).

[4] V. Holubec, J. Stat. Mech: Theory Exp. **2014**, P05022 (2014).

[5] V. Holubec and A. Ryabov, Phys. Rev. E **92**, 052125 (2015).

[6] M. Esposito, R. Kawai, K. Lindenberg, and C. Van den Broeck, Phys. Rev. Lett. **105**, 150603 (2010).

[7] V. Holubec, K. Kroy, and S. Steffenoni, arXiv preprint arXiv:1804.01285 (2018).

[8] V. Holubec and A. Ryabov, Phys. Rev. E **96**, 062107 (2017).

[9] A. del Campo, Phys. Rev. Lett. **111**, 100502 (2013).

[10] E. Torrontegui, S. Ibez, S. Martnez-Garaot, M. Modugno, A. del Campo, D. Gury-Odelin, A. Ruschhaupt, X. Chen, and J. G. Muga, in *Advances in Atomic, Molecular, and Optical Physics*, Advances In Atomic, Molecular, and Optical Physics, Vol. 62, edited by E. Arimondo, P. R. Berman, and C. C. Lin (Academic Press, 2013) pp. 117 – 169.

[11] Z. C. Tu, Phys. Rev. E **89**, 052148 (2014).

[12] G. Li, H. T. Quan, and Z. C. Tu, Phys. Rev. E **96**, 012144 (2017).

[13] I. A. Martínez, A. Petrosyan, D. Guéry-Odelin, E. Trizac, and S. Ciliberto, Nature physics **12**, 843 (2016).

[14] N. Shiraishi and H. Tajima, Phys. Rev. E **96**, 022138 (2017).
